# Supplementary material for: Precision-Machine Learning for the Matrix Element Method
Source: arXiv:2310.07752 source file (2024-10-03)

$\alpha = 0^\circ$ , 400 events

$-2\log L(\alpha)$

— hard  
— Transfermer  
— Parallel TFusion

-10

0

10

CP-phase  $\alpha$  [ $^\circ$ ]

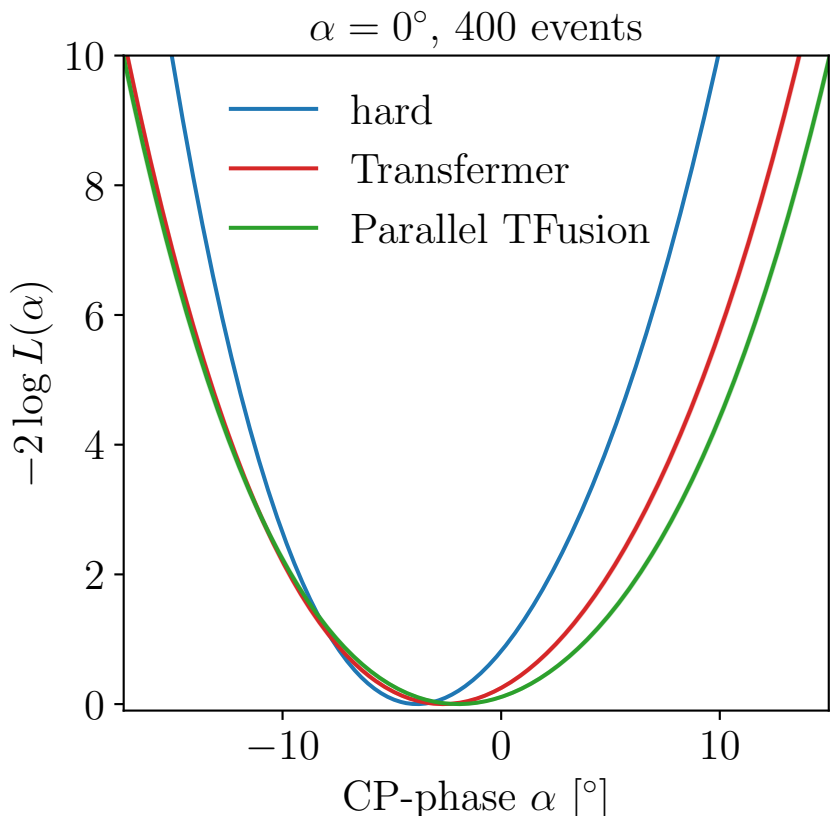

$\alpha = 45^\circ$ , 400 events

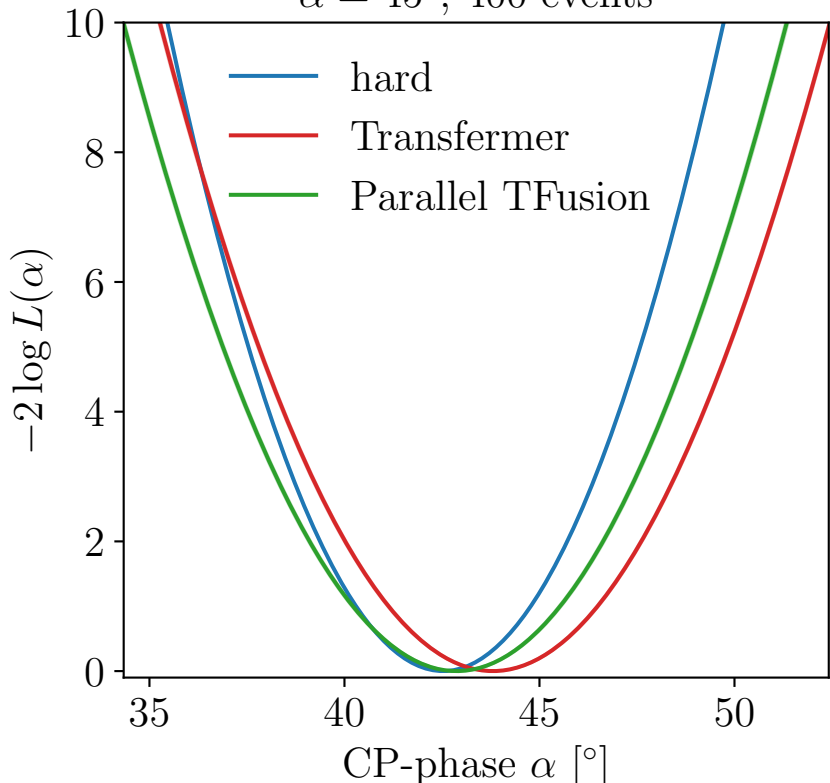

$\alpha = 90^\circ$ , 400 events

$-2\log L(\alpha)$

hard  
Transformer  
Parallel TFusion

0

2

4

6

8

10

80

90

100

110

CP-phase  $\alpha$  [ $^\circ$ ]

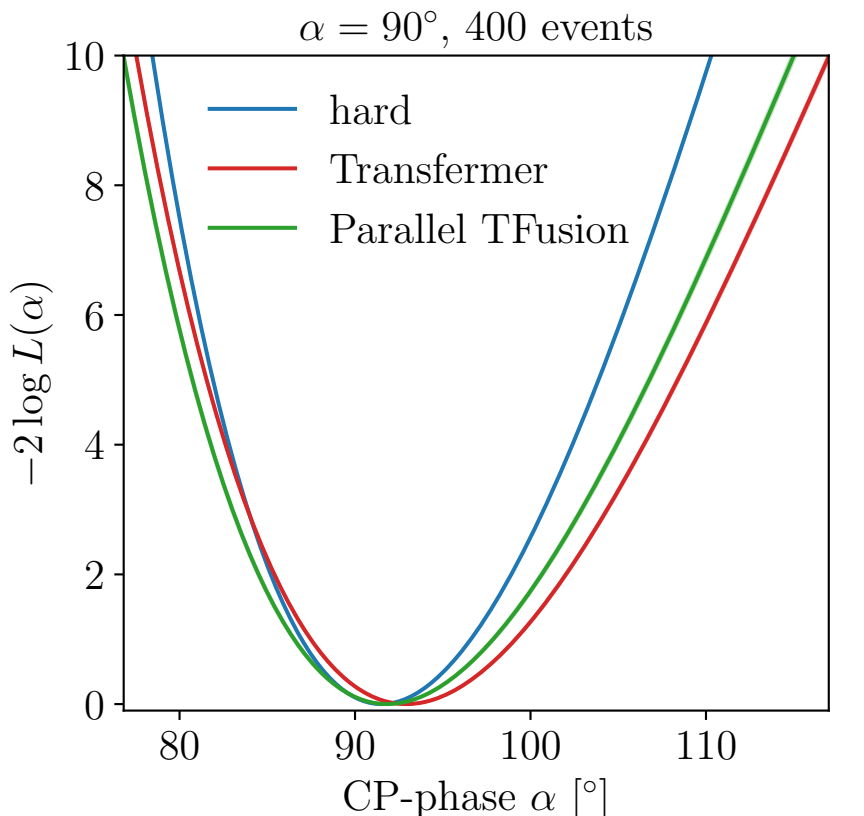

Supplement: Supplementary file 1 [file likelihoods_appendix.pdf]
